# Supplementary material for: Point-Selection Fine-Tuning Framework for Robust Point Cloud Classification
Source: arXiv:2607.19711 source file (2026-07-22)
Supplement: Supplementary file 1 [file supp.tex]

\documentclass[runningheads]{llncs}

\usepackage{booktabs}
\usepackage{array}
\usepackage{float}
\usepackage{multirow}
\usepackage{siunitx}
\usepackage[T1]{fontenc}
\usepackage[hidelinks]{hyperref}

\newcolumntype{L}[1]{>{\raggedright\arraybackslash}p{#1}}
\newcolumntype{C}[1]{>{\centering\arraybackslash}p{#1}}
\newcolumntype{A}{S[table-format=2.1]}
\newcolumntype{E}{S[table-format=1.3]}
\newcolumntype{R}{S[table-format=2.1]}

\sisetup{
  detect-family=true,
  detect-weight=true,
  group-digits=false,
  table-number-alignment=center
}

\setlength{\textfloatsep}{8pt plus 2pt minus 2pt}
\setlength{\floatsep}{6pt plus 2pt minus 2pt}
\setlength{\intextsep}{6pt plus 2pt minus 2pt}
\setlength{\abovecaptionskip}{4pt}
\setlength{\belowcaptionskip}{2pt}
\setlength{\aboverulesep}{0.25ex}
\setlength{\belowrulesep}{0.40ex}
\raggedbottom

\begin{document}
\input{sections/x_suppl}

\bibliographystyle{splncs04}
\bibliography{references}
\end{document}
